# Supplementary material for: SHIRO: Soft Hierarchical Reinforcement Learning
Source: arXiv:2212.12786 source file (2022-12-24)
Supplement: Supplementary file 1 [file covid_19.tex]

\section*{COVID-19 Impact}
Due to the COVID-19 Pandemic, as well as the fact that the authors were working in different countries, the extent of our experiments was limited to only include simulated robot experiments. The main deficiencies of our work compared to real-world experiments is that the environments in which we tested on (simulated robot navigation tasks) have a simpler model to learn from than the real world, which may suggest that deployment on a real robot would be significantly more challenging.

However, we believe that the evaluation methodology is sufficient and would transfer to a real robot for the reasons listed below:

\begin{enumerate}

  \item \textbf{Our method can be viewed as a hierarchical extension of SAC, and SAC has proven to work well in different real robot scenarios:} Our work enables us to view our method as SAC through our theoretical contribution, and empirically performs much better than SAC (which is unable to complete the long-horizon tasks). Previous work in \cite{haarnoja2018soft} applied SAC with a learned temperature on a $9$-DoF dexterous hand manipulation task and learning gaits on an underactuated, $8$-DoF Minitaur robot. The first task also required visual-input, but SAC is still able to complete the task more than twice as fast as other algorithms such as PPO. SAC also quickly learns the second task, and the learned policies on the Minitaur are even able to generalize to different terrains. Thus, we believe that our work, which quickly learned with the $8$-DoF simulated robot, will be able to learn real robot policies as well and longer-horizon tasks.
  
  \item \textbf{A hierarchical RL method similar to ours has succeeded on long-horizon real robot tasks:} The work in \cite{nachum2020multi} learns hierarchical policies for long-horizon locomotion. Specifically, their method uses temporally abstracted goal-conditioned HRL with nearly the same architecture as HIRO (with high-level actions being in $x, y$ space). They first train the low-level policy on random goals, then train the high-level policy. We believe that our method would be able to learn similar tasks faster because we can train both policies concurrently \textit{while} improving the low-level policy via random sub-goals.

  \item \textbf{Our method targets data efficiency:} The biggest advantage of our proposed work is that it is even more data efficient than prior state-of-the-art. Especially with real robots, this sample efficiency is highly desirable.
  \item {\textbf{Our method learns a more robust low-level:}} Our results empirically demonstrate that the low-level agent is able to learn to more closer reach sub-goals when entropy on the high-level agent is maximized. We posit that this is beneficial for real robots, where increased robustness will assist in the challenging dynamics.

\end{enumerate}

In order to experimentally validate the method with real data, we will test our methods on a robot manipulator -- namely, the Franka Emika Panda, a $7$-DoF collaborative robot -- on a reach and pick and place (a simple block) task. For the reach task, the robot will need to generate subgoals that allow it to move to the goal; for the pick and place task, the manipulator needs to plan how to move to a target, pick it up, and move it to a desired goal.  Furthermore, we plan to validate our work on the Minitaur robot on a simple maze and push task.
